# Supplementary material for: In situ and operando laboratory X-ray absorption spectroscopy at high temperature and controlled gas atmosphere with a plug-flow fixed-bed cell
Source: arXiv:2601.11298 ancillary file (2026-04-21)
Supplement: Supplementary file 1 [file SI.pdf]

Supplementary Information:

# *In situ* and *operando* laboratory X-ray absorption spectroscopy at high temperature and controlled gas atmosphere with a plug-flow fixed-bed cell

Sebastian Praetz,[*a‡] Emiliano Dal Molin,[b‡] Delf Kober,[b] Marko Tesic,[a] Christopher Schlesiger,[a] Peter Kraus,[c] Julian T. Müller,[b] Jyothilakshmi Ravi Aswin,[d] Daniel Grötzsch,[a] Maged F. Bekheet,[b] Albert Gili,[e] Aleksander Gurlo,[b] and Birgit Kanngießer[a]

[a] *Technische Universität Berlin, Institute of Physics and Anstronomy, Sekr. EW 3-1, Hardenbergstraße 36, 10623 Berlin, Germany. E-mail: sebastian.praetz@tu-berlin.de*

[b] *Technische Universität Berlin, Faculty III Process Sciences, Institute of Materials Science and Technology, Chair of Advanced Ceramic Materials, Hardenbergstr. 40, 10623 Berlin, Germany.*

[d] *Technische Universität Berlin, Conductivity and Catalysis Lab, Hardenbergstr. 40, 10623 Berlin, Germany.*

[d] *Helmholtz-Zentrum Berlin, Department Atomic-Scale Dynamics in Light-Energy Conversion, 14109 Berlin, Germany.*

[e] *Helmholtz-Zentrum Berlin für Materialien und Energie, 14109 Berlin, Germany.*

‡ These authors contributed equally to this work

This is the supplementary information for the work titled "*In situ* and *operando* laboratory X-ray absorption spectroscopy at high temperature and controlled gas atmosphere with a plug-flow fixed-bed cell" uploaded as a preprint on arXiv. It provides additional details on the experimental setup, including the von Hámos configuration for XAS measurements and the IR tube furnace plug-flow reactor cell, as well as extended characterization of the catalysts by XRD and XRF. Furthermore, it contains supplementary XAS measurements and analysis (capillary versus pellet spectra, *in situ* oxidation of MnO, *operando* and *in situ* studies of 20-NiO/COK-12 with linear combination fitting and normalized data), gas chromatography measurements, additional post-reduction *operando* experiments, and information on an X-ray source optimized for 30 keV.

## Contents

1 Experimetnal setup 2
1.1 Von Hámos Setup for XAS measurements . . . 2
1.2 IR tube furnace reactor cell . . . 3

2 XRD measurement of synthesized 5 % Ni/MnO catalyst 5

3 XRF measurements of 20-NiO/COK-12 5

4 Supplementary XAS measurements and analysis 6
4.1 Capillary spectra and normalized comparison with pellet samples . . . 6
4.2 *In situ* Oxidation of MnO . . . 9
4.2.1 Linear combination fitting . . . 9
4.3 *Operando* measurements of 20-NiO/COK-12 . . . 12
4.3.1 Linear combination fitting . . . 16
4.4 *In situ* Reduction of 20-NiO/COK-12 . . . 18
4.4.1 Raw $\mu Q$ spectra . . . 18
4.4.2 Normalized data . . . 19
4.4.3 Linear combination fitting . . . 20

5 GC measurements 21

6 Additional post-reduction operando experiments 22

7 X-ray source optimized for 30 keV 23

# 1 Experimetnal setup

## 1.1 Von Hámos Setup for XAS measurements

Figure S1 shows the complete von Hámos X-ray absorption spectroscopy setup. From right to left, the X-rays first pass through a shutter and then transmit through the sample cell. After exiting the cell, the beam passes through an adjustable slit before being projected onto the cylindrically curved HAPG crystal optic. The dispersed X-rays are then reflected onto an area detector. To minimize absorption by air, the beam paths between the X-ray source and the optic, as well as between the optic and the detector, are enclosed in two adjustable vacuum tubes.

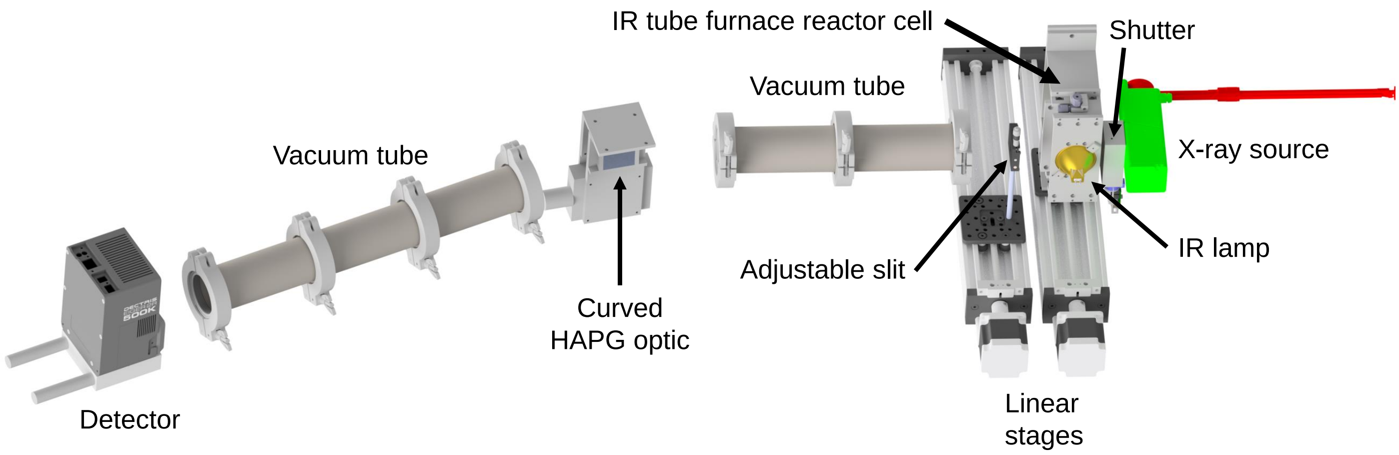


Fig. S1 CAD model of the modified von Hámos setup for XAS measurement. All the relevant components are displayed, including the orientation of the IR tube furnace reactor cell (containing the sample in a capillary) in the von Hámos setup.

## 1.2 IR tube furnace reactor cell

This section shows in detail the infrared (IR) tube furnace reactor cell setup. Fig. S2 shows the complete reactor cell with the assembled transport plate. An explosion view of the transport cell is shown in Fig. S3. In Fig. S4 a technical drawing of the SiC tube is shown, with the modified entrance and exist slit of 4 mm each, compared to the version used in Bischoff *et al.* [1]

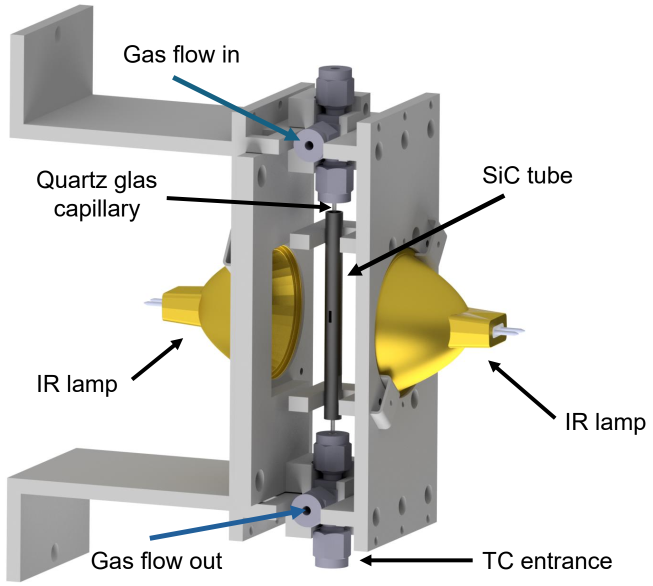


Fig. S2 CAD model of the IR tube furnace reactor cell. Two IR lamps heating the SiC tube, which surrounds the loaded quartz glass capillary.

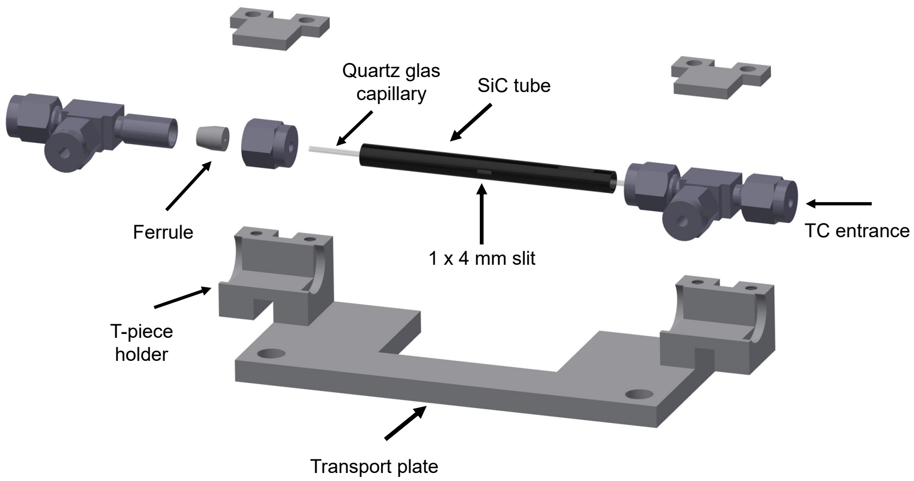


Fig. S3 Exploded view of the transport plate, showing the components used to assemble the loaded capillary. The capillary is sealed airtight to the T-pieces using 1/8" Vespel/Graphite ferrules. After assembly, the T-pieces are secured to the transport plate to prevent movement of the system.

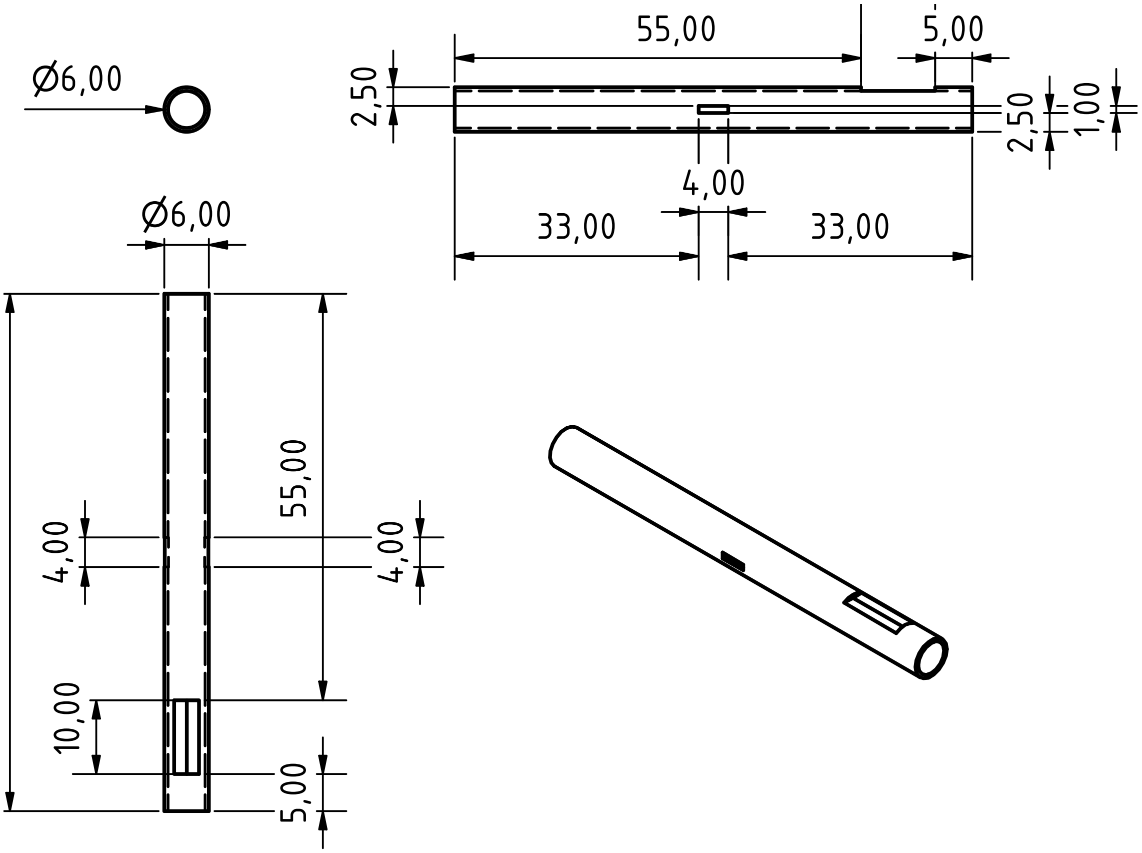


Fig. S4 Technical drawing of the SiC tube, which functions as the furnace, including detailed information on its geometry and cutouts. The SiC tube has 4 mm slits on both sides to allow X-rays to pass through. All numbers given are in mm.

## 2 XRD measurement of synthesized 5 % Ni/MnO catalyst

Fig. S5 shows the diffraction pattern of the synthesized 5 % Ni/MnO catalyst before (XXMD11_D1MD11, blue curve) and after (XXMD12_D1MD12, black curve) reduction with 5 % $H_2$ in Ar at 500 °C for at least 60 min to reduce NiO/$Mn_2O_3$ to Ni/MnO.

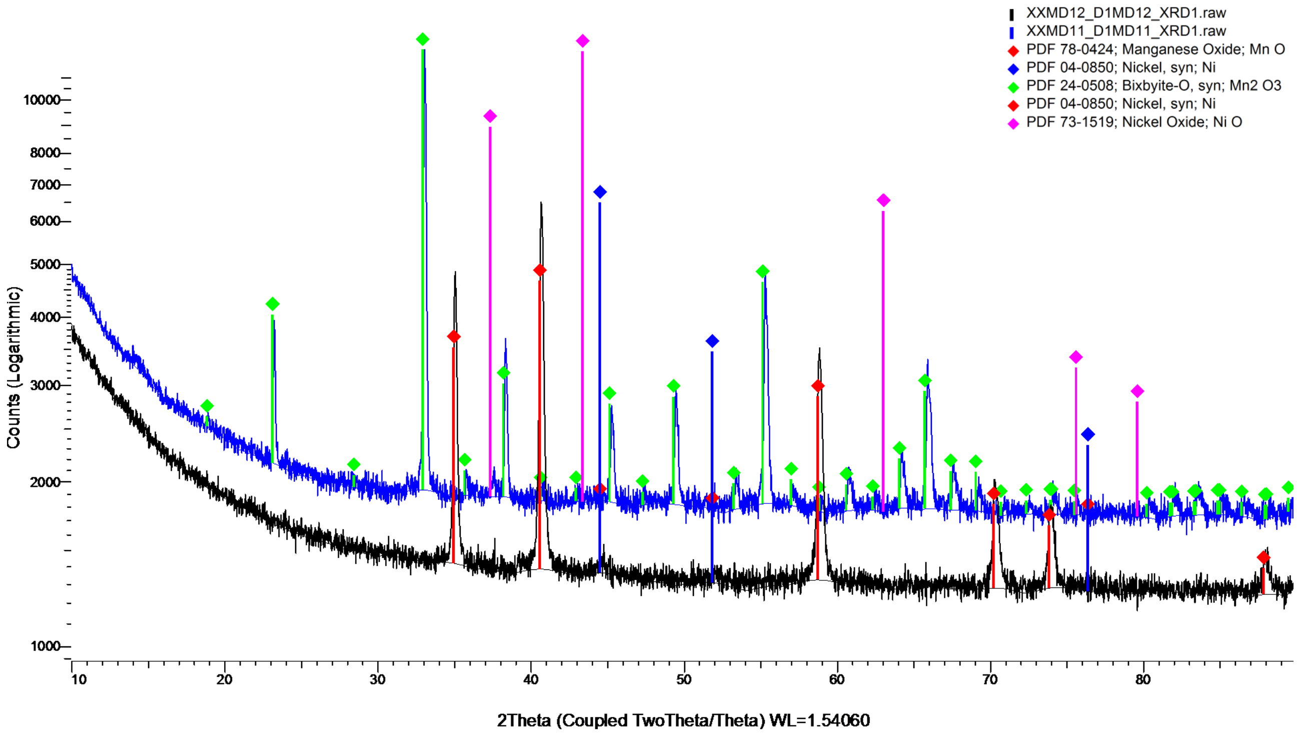


Fig. S5 XRD measurement of the synthesized 5 % Ni/MnO catalyst before (XXMD11_D1MD11, blue curve) and after (XXMD12_D1MD12, black curve) reduction with 5 % $H_2$ in Ar at 500 °C for at least 60 min to reduce NiO/$Mn_2O_3$ to Ni/MnO.

## 3 XRF measurements of 20-NiO/COK-12

Quantitative X-ray fluorescence (XRF) on the 20-NiO/COK-12 catalyst after calcination was performed using a *FISCHERSCOPE® X-RAY XDV®-SDD* spectrometer equipped with a microfocus tungsten X-ray tube and a beryllium window. Measurements were carried out at 50 kV without any primary filter. Component analysis revealed 20.2 wt.% NiO and 79.8 wt.% $SiO_2$, corresponding to approximately 15.8 wt.% Ni content in the catalyst.

## 4 Supplementary XAS measurements and analysis

### 4.1 Capillary spectra and normalized comparison with pellet samples

The unnormalized spectra of different materials measured while loaded in a capillary at different absorption K-edges (Mn, Ni, Se and Zr) are shown in Fig. S6–S9. The normalized spectra in comparison with the material prepared as a free standing pellet are presented in Fig. S10 and S11.

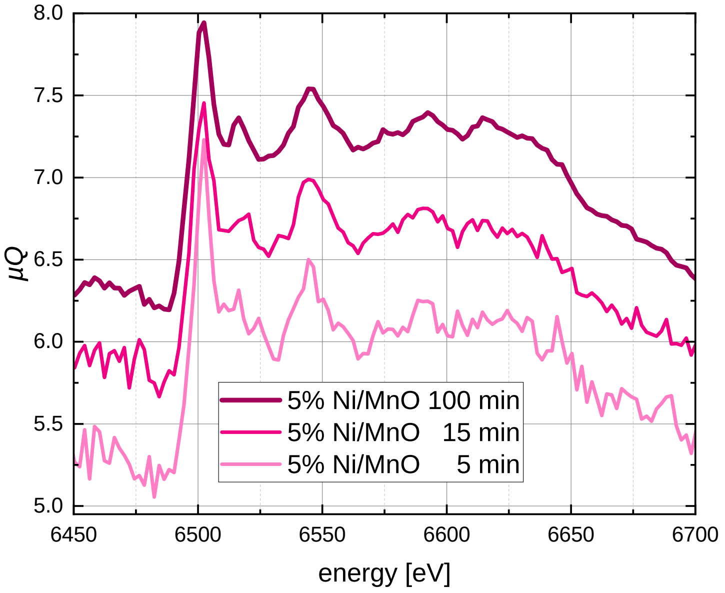


Fig. S6 Mn K-edge XAS spectrum of 5 %Ni/$MnO_2$ measured in a 1.0/0.8-capillary at RT for different measurement times.

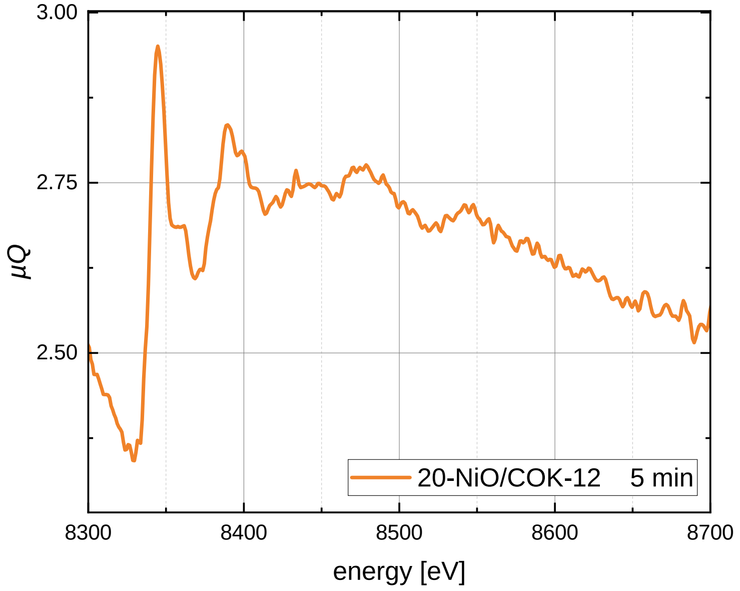


Fig. S7 Ni K-edge XAS spectrum of 20-NiO/COK-12 measured in a 1.0/0.8-capillary at RT. The measurement time was 5 min (300 s).

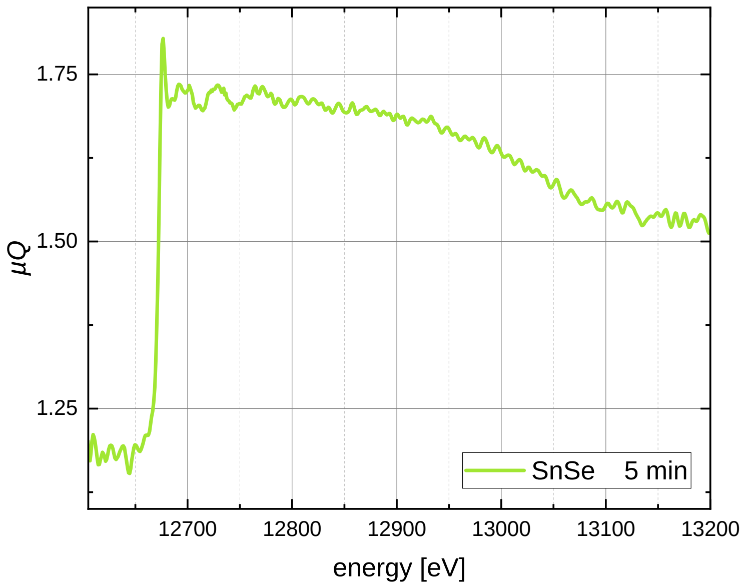


Fig. S8 Se K-edge XAS spectrum of SnSe measured in a 1.0/0.8-capillary at RT. The measurement time was 5 min (300 s).

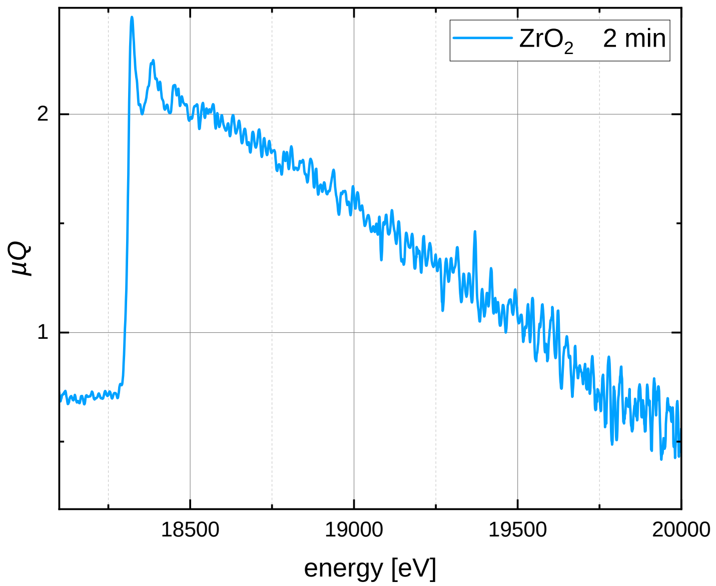


Fig. S9 Zr K-edge XAS spectrum of $ZrO_2$ measured in a 1.5/1.0-capillary at RT. The measurement time was 2 min (120 s).

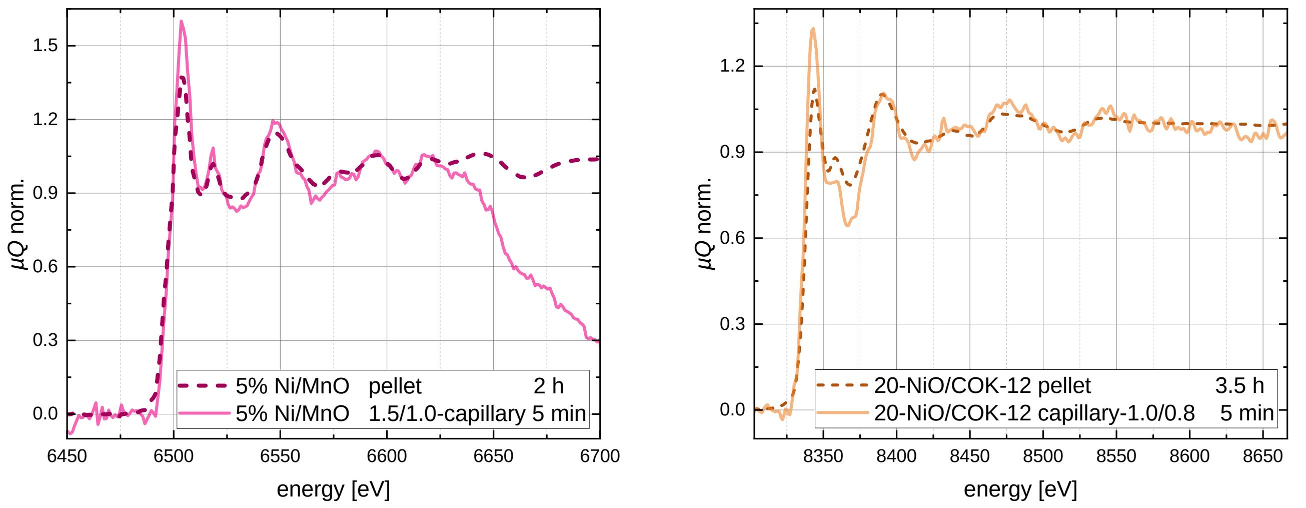


Fig. S10 Normalized Mn K-egde XAS spectra of 5 % Ni/$MnO_2$ in a 1.0/0.8-capillary in comparison to a pellet sample of the same material (left) and Ni K-edge spectra of 20-NiO/COK-12 in a 1.0/0.8-capillary in comparison to pellet sample of the same material (right).

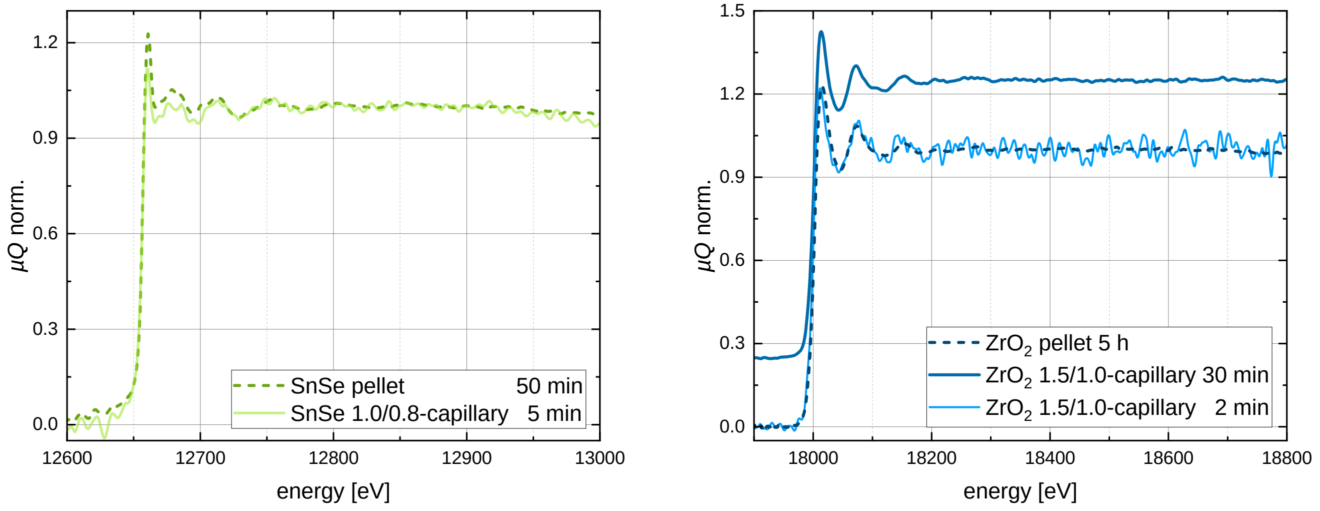


Fig. S11 Normalized Se K-egde XAS spectra of SnSe in a 1.0/0.8-capillary in comparison to a pellet sample of the same material (left) and Zr K-edge spectra of $ZrO_2$ in a 1.5/1.0-capillary in comparison to pellet sample of the same material (right).

## 4.2 *In situ* Oxidation of MnO

### 4.2.1 Linear combination fitting

Fig. S12–S14 show the linear combination fits (LCF) of 5 % Ni/MnO measured at different temperatures *in situ*. The LCF at 100 °C is not included, as it does not differ from the RT spectrum within the uncertainties of the fit. The fitting range covers 20 eV before and 125 eV beyond the edge position of the spectra. Fig. S15 presents the fitted component fractions as a function of temperature. All fitting results including R-factor, $\chi^2$ and $\chi^2_\nu$ are listed in Table S1.

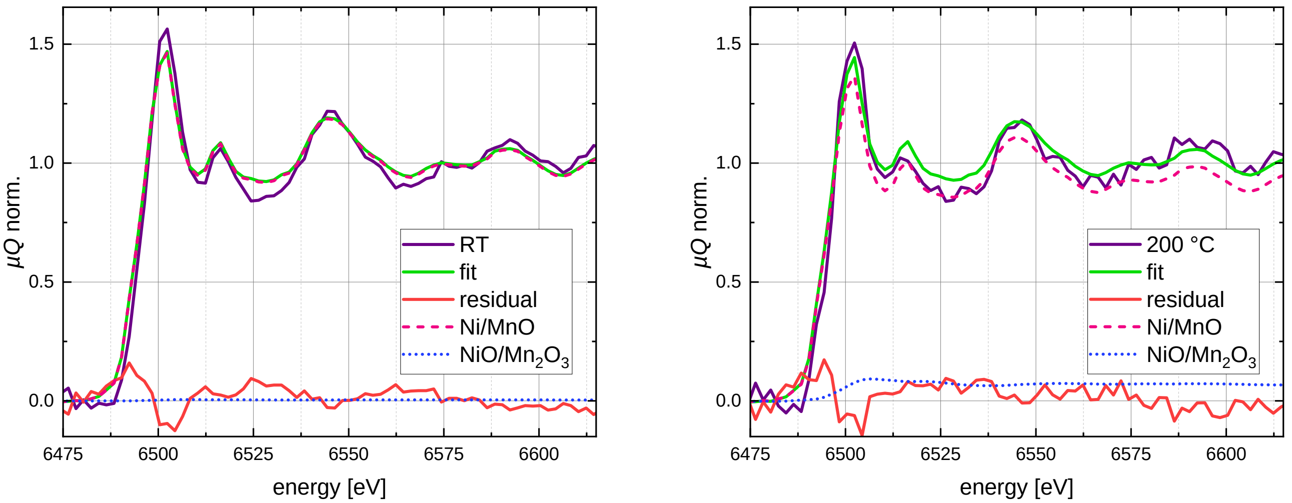


Fig. S12 Linear combination fitting (LCF) of the *in situ* Ni/MnO Mn K-edge XAS measurement at RT (left) before heating and at 200 °C (right).

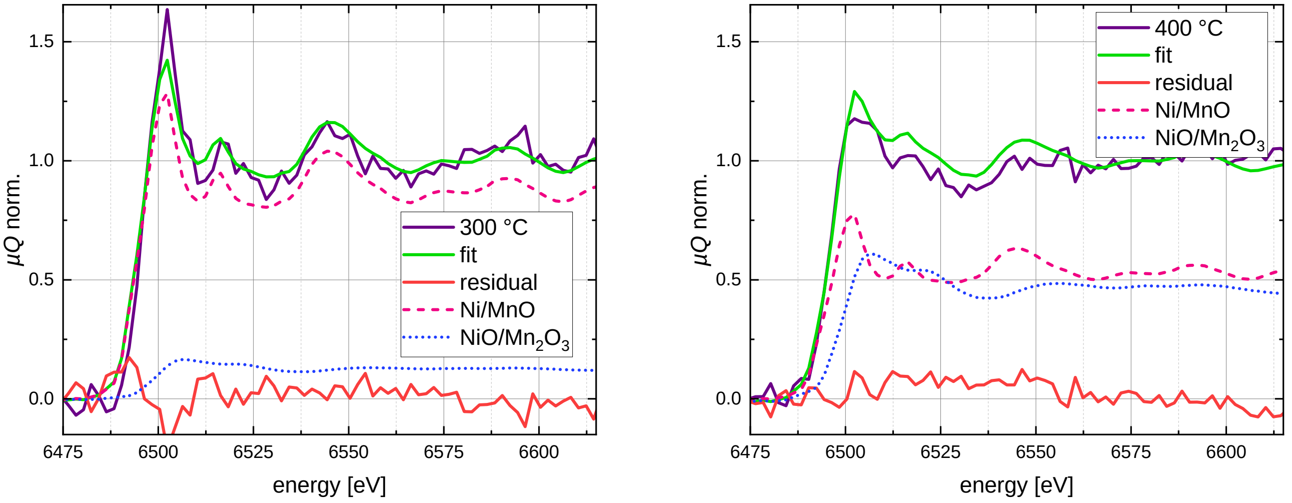


Fig. S13 Linear combination fitting (LCF) of the *in situ* Ni/MnO Mn K-edge XAS measurement at 300 °C (left) and at 400 °C (right).

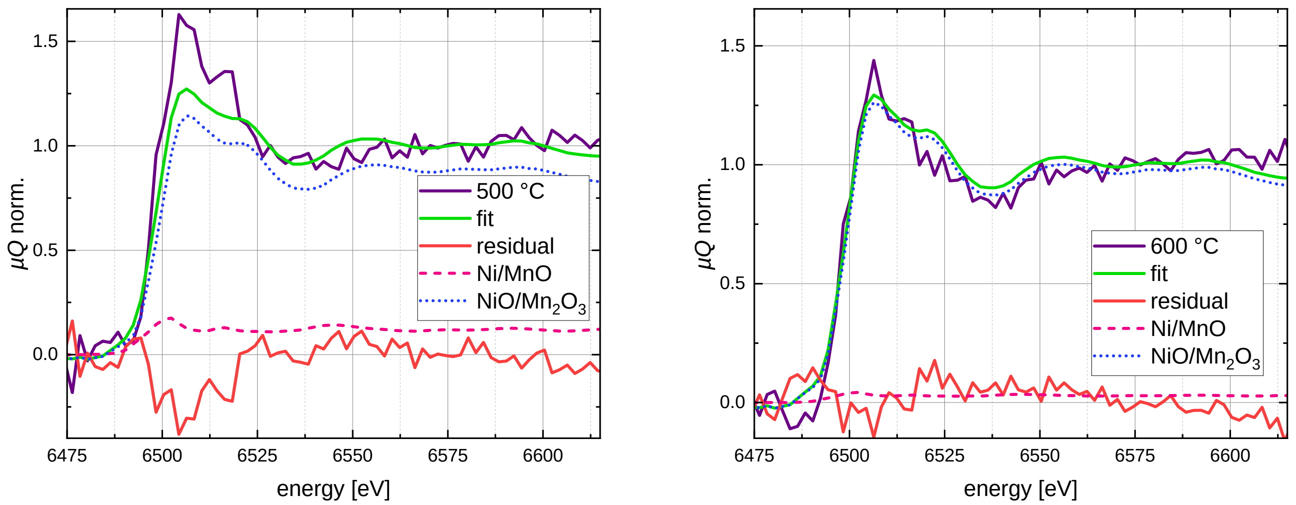


Fig. S14 Linear combination fitting (LCF) of the *in situ* Ni/MnO Mn K-edge XAS measurement at 500 °C (left) and at 600 °C (right).

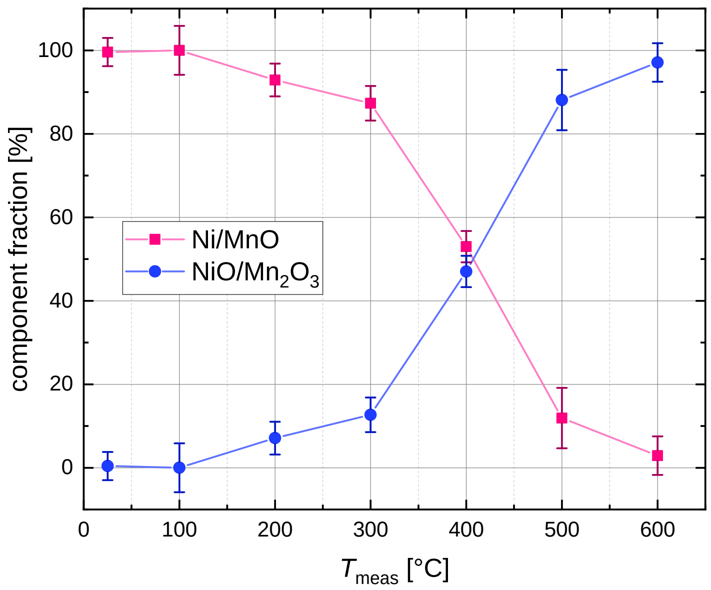


Fig. S15 Component fraction during *in situ* resulting from the LCF (Fig. S12–S14). The references used for the LCF are Ni/MnO and NiO/$Mn_2O_3$.

Table S1 LCF results at different temperatures $T$ using Ni/MnO and NiO/$Mn_2O_3$ as standards. Uncertainties are given as $\pm$ values. Reduced chi-square ($\chi_v^2$) and raw chi-square ($\chi^2$) values are reported to assess the fit quality, with $\chi_v^2$ accounting for the degrees of freedom.

| $T$ [°C] | R-factor | $\chi_v^2$ | $\chi^2$ | Ni/MnO | NiO/$Mn_2O_3$ |
|---|---|---|---|---|---|
| 25 | 0.0222 | 0.00256 | 0.18691 | 1.00 ± 0.04 | 0.00 ± 0.04 |
| 100 | 0.0579 | 0.00769 | 0.56133 | 1.00 ± 0.06 | 0.00 ± 0.06 |
| 200 | 0.0306 | 0.00346 | 0.25221 | 0.93 ± 0.04 | 0.07 ± 0.04 |
| 300 | 0.0330 | 0.00385 | 0.28113 | 0.87 ± 0.05 | 0.13 ± 0.05 |
| 400 | 0.0337 | 0.00315 | 0.22986 | 0.53 ± 0.04 | 0.47 ± 0.04 |
| 500 | 0.0886 | 0.01167 | 0.85190 | 0.12 ± 0.08 | 0.88 ± 0.08 |
| 600 | 0.0373 | 0.00477 | 0.34836 | 0.03 ± 0.05 | 0.97 ± 0.05 |

### 4.3 *Operando* measurements of 20-NiO/COK-12

The raw *operando* XAS measurements of 20-NiO/COK-12 are shown in Fig. S16 (before activation), Fig. S17 (during activation/reduction), and Fig. S19 (after activation). Fig. S20 presents the LCF result of the final spectrum at 600 °C, using the fitting different ranges (wide: complete spectrum, mid: EXAFS region and narrow: XANES/edge and white line) applied to all spectra during heating and cooling. The resulting component fractions as a function of time are shown in Fig. S21.

Fig. S18 is comparing the NiO reference spectra with 20-NiO/COK-12 sample highlighting the difference – indicated by the residual – caused by the metal–support interactions (MSIs). Furthermore, the edge position determined by the half-step and first maximum of the first derivative methods are shown in Table S2.

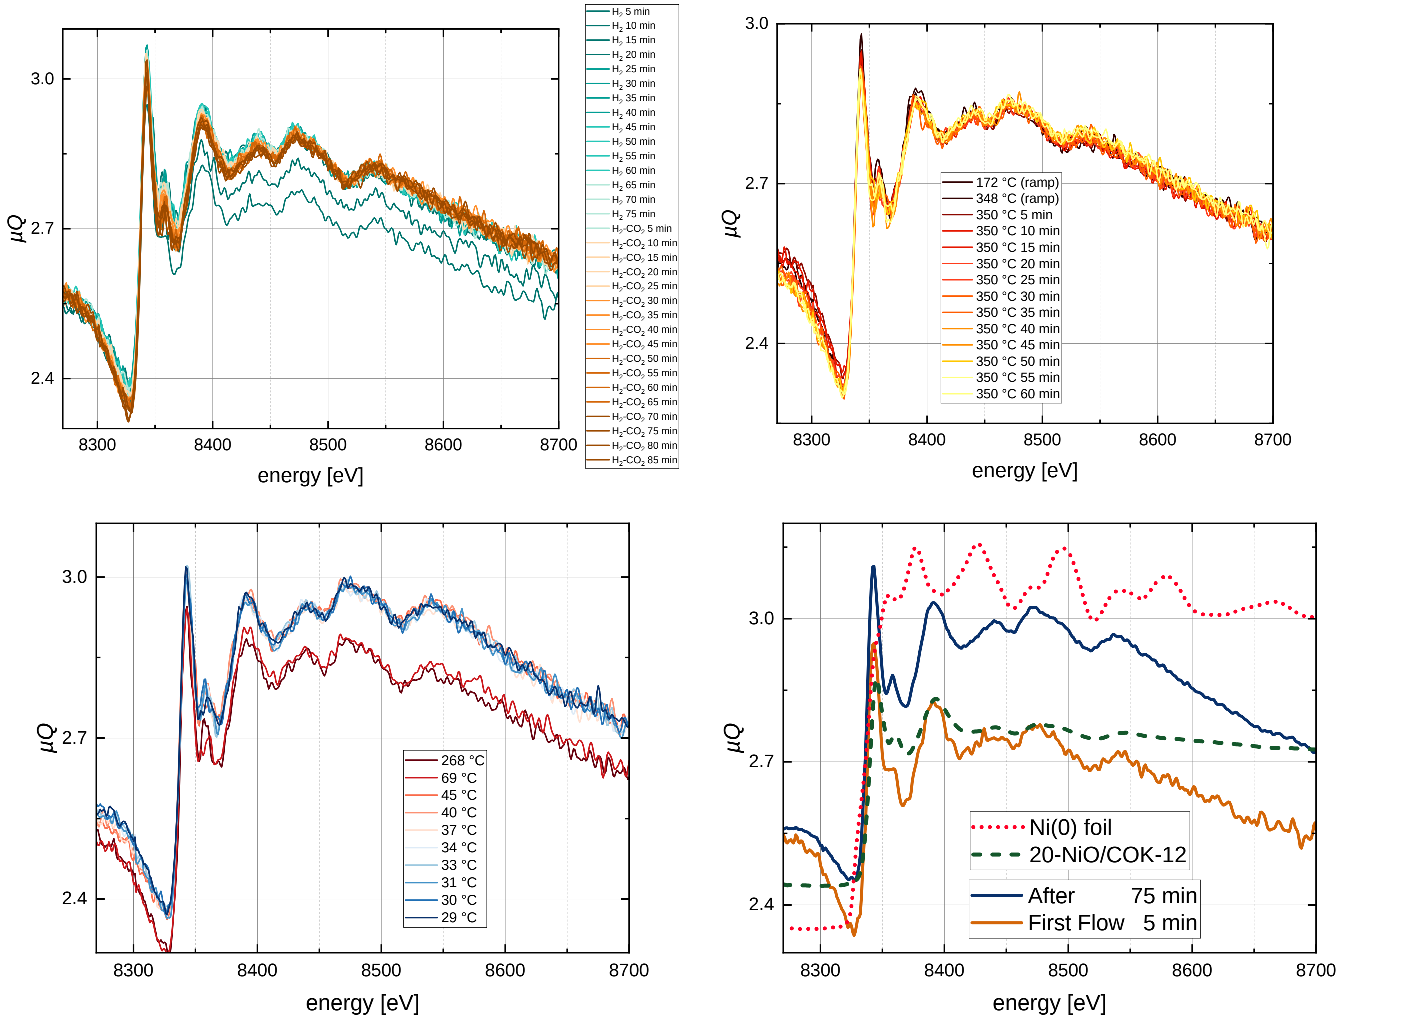


Fig. S16 Raw *operando* XAS spectra under reaction condition, with $H_2$ (17.2 mL/min 5 % $H_2$/Ar at NTP)) and $CO_2$ (0.6 mL/min $CO_2$ at NTP)) gas flow in the ratio of 4:1 at 350 °C, before activation of the catalyst. Top left: during gas flow setup at RT. Top right: during heating from RT to 350 °C. Bottom left: during cool down to RT. Bottom right: comparison of first spectrum during flow and long measurement after the *operando* measurement alongside the reference spectra of a Ni metal-foil and the material 20-NiO/COK-12 prepared as pellet.

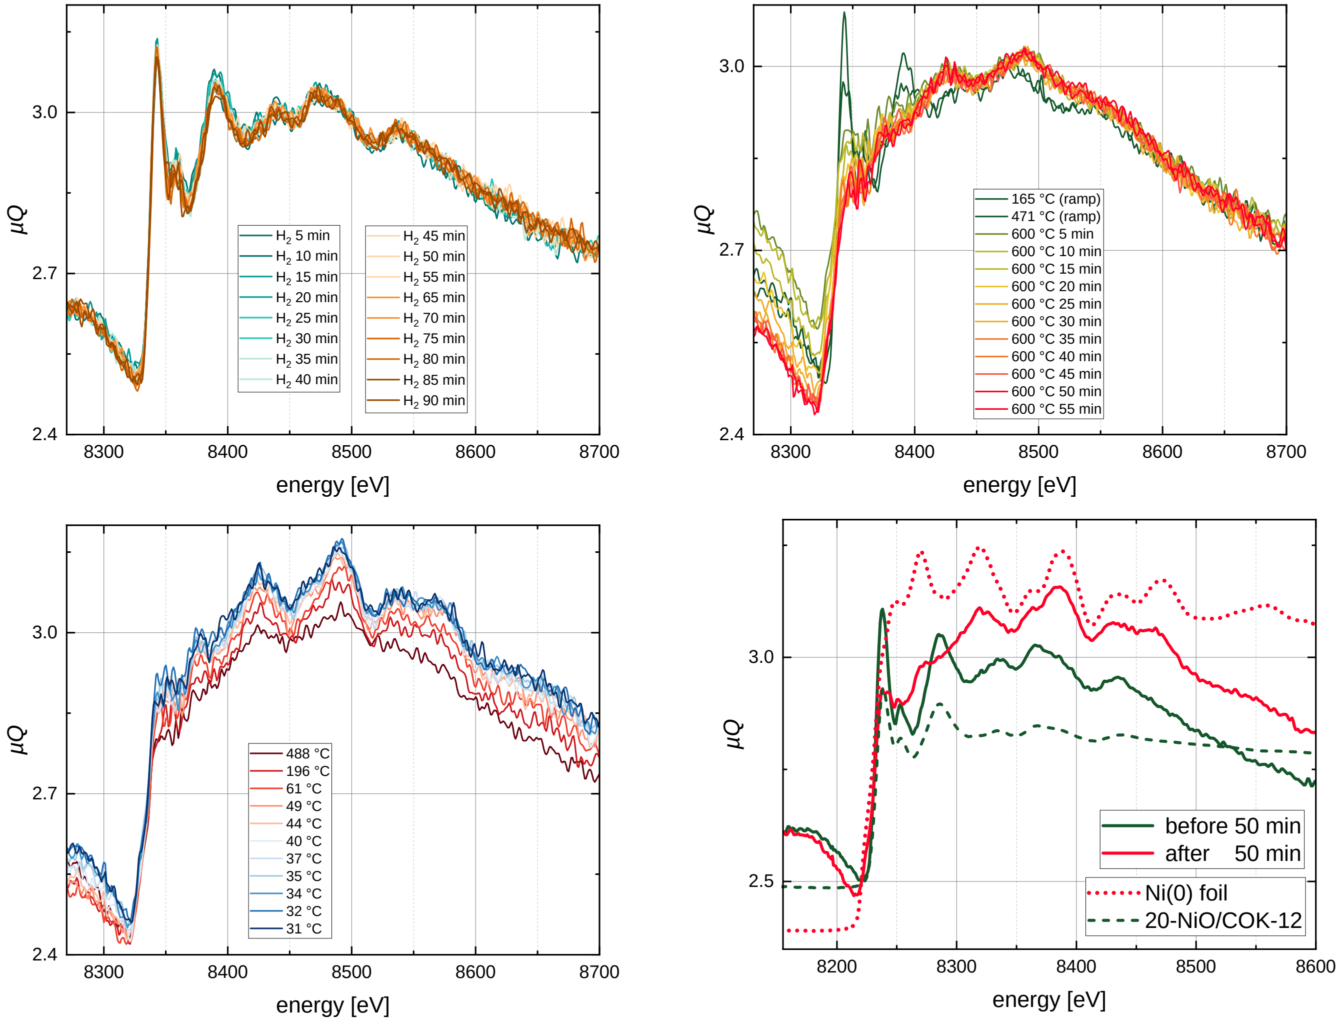


Fig. S17 Raw *operando* XAS spectra during the reduction/activation of the catalyst. Top left: during gas flow setup at RT. Top right: during heating from RT to 600 °C. Bottom left: during cool down to RT. Bottom right: Comparison before and after reduction with $H_2$ flow at 600 °C.

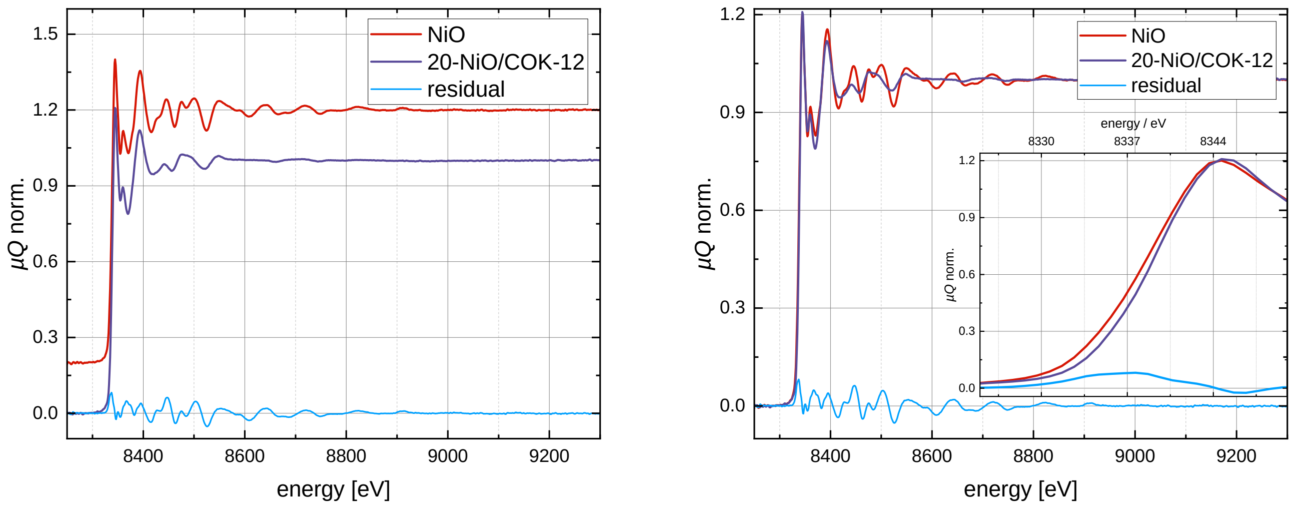


Fig. S18 Normalized XAS spectra of the reference sample NiO and 20-NiO/COK-12 before reduction, both samples prepared as pellets. Left: shows both spectra with an offset. Right: direct comparison, including an inset with the edge region showing a slight shift of 20-NiO/COK-12 towards higher energies.

Table S2 Comparison of Ni K-edge positions of the measured references and 20-NiO/COK-12 determined using the half-step and first maximum of the first derivative methods.

| **Sample** | **Half-step [eV]** | **Second derivative [eV]** |
|---|---|---|
| Ni foil | 8337.48 $\pm$ 0.03 | 8327.21 $\pm$ 0.08 |
| NiO | 8336.95 $\pm$ 0.04 | 8339.22 $\pm$ 0.14 |
| 20-NiO/COK-12 | 8337.71 $\pm$ 0.04 | 8338.56 $\pm$ 0.21 |

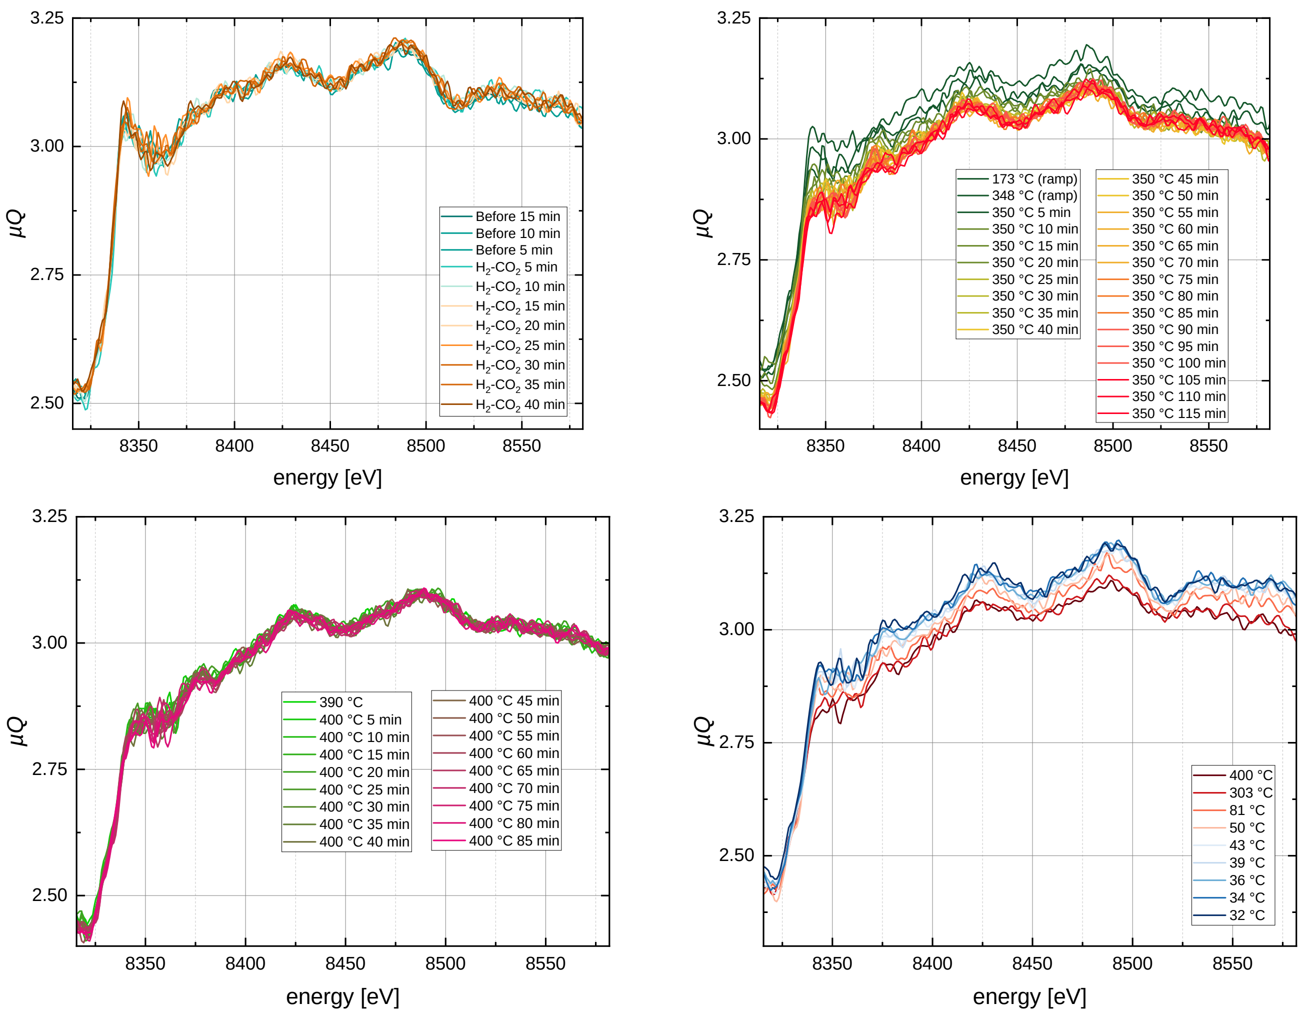


Fig. S19 Raw *operando* XAS spectra under reaction condition, with $H_2$ and $CO_2$ gas flow in the ratio of 4:1 at 350 °C, after reduction/activation of the catalyst. Top left: during gas flow setup at RT. Top right: during heating from RT to 350 °C. Bottom left: further increasing the temperature from 350 °C to 400 °C. Bottom right: during cool down from 400 °C to RT.

### 4.3.1 Linear combination fitting

Fig. S20 shows the three different fitting ranges used for the LCF applied to the *operando* XAS measurement during the reduction of 20-NiO/COK-12. The LCF with these fitting ranges was applied to the entire measurement, covering the heating from RT to 600 °C (ramp), the isothermal hold at 600 °C for about 50 minutes (hold) and the subsequent cooling down to RT. The corresponding component fraction plots are presented in Fig. S21.

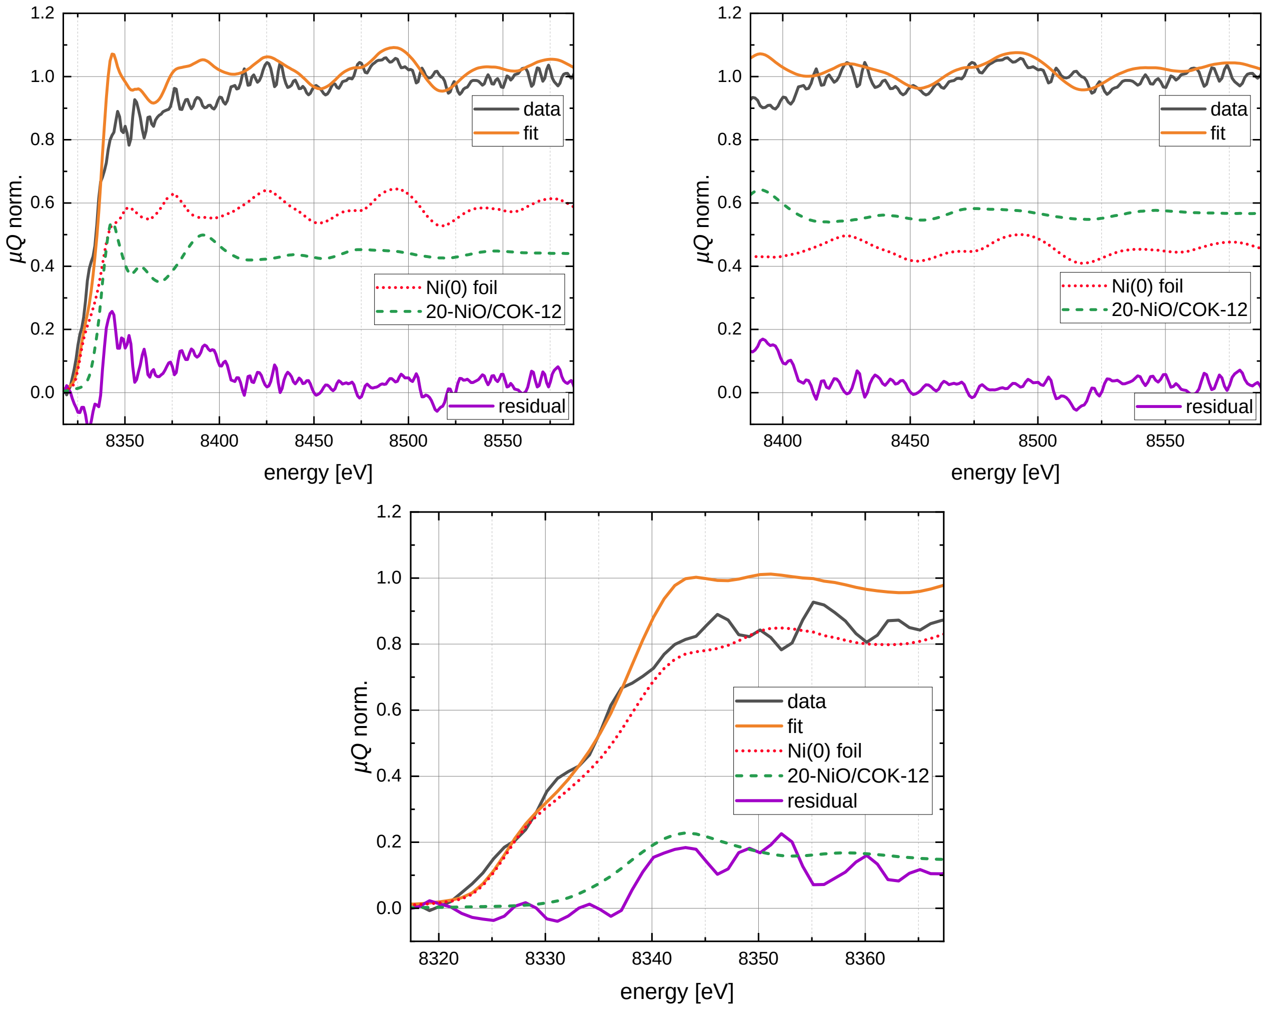


Fig. S20 LCF of the last *operando* spectrum at 600 °C alongside the fitted component fraction and the residual of fit and data for the three different fitting ranges. Top left: wide range covering 20 eV before to 250 eV beyond the edge. Top right: mid range covering 50 eV to 250 eV beyond the edge. Bottom: narrow edge covering 20 eV before to 30 eV beyond the edge.

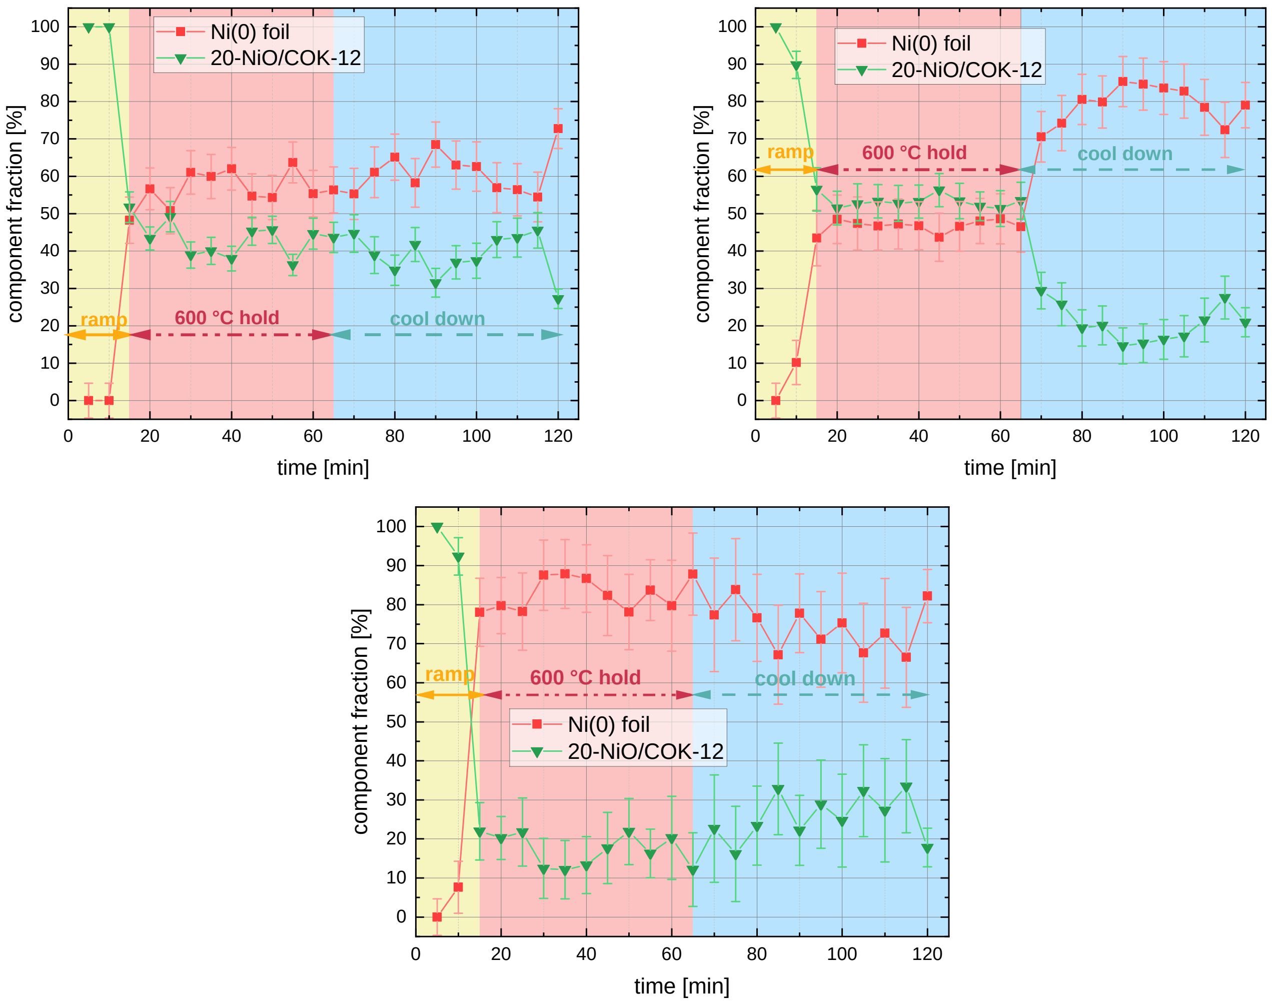


Fig. S21 Fractional component of the LCF of the complete reduction measurement from starting heating (ramp) to cool down, after holding the temperature 600 °C for 55 minutes, for the three different fitting ranges. Top left: wide range covering 20 eV before to 250 eV beyond the edge. Top right: mid range covering 50 eV to 250 eV beyond the edge. Bottom: narrow edge covering 20 eV before to 30 eV beyond the edge.

### 4.4 *In situ* Reduction of 20-NiO/COK-12

In the following Sections 4.4.1 – 4.4.3 and figures the raw (Fig. S22) and normalized spectra (Fig. S23) of the *in situ* measurement of 20-NiO/COK-12 are presented alongside the component fraction plot (Fig. S24) obtained by LCF.

#### 4.4.1 Raw $\mu Q$ spectra

In Fig. S22 the raw spectra of the *in situ* measurement of the reduction of 20-NiO/COK-12 is shown.

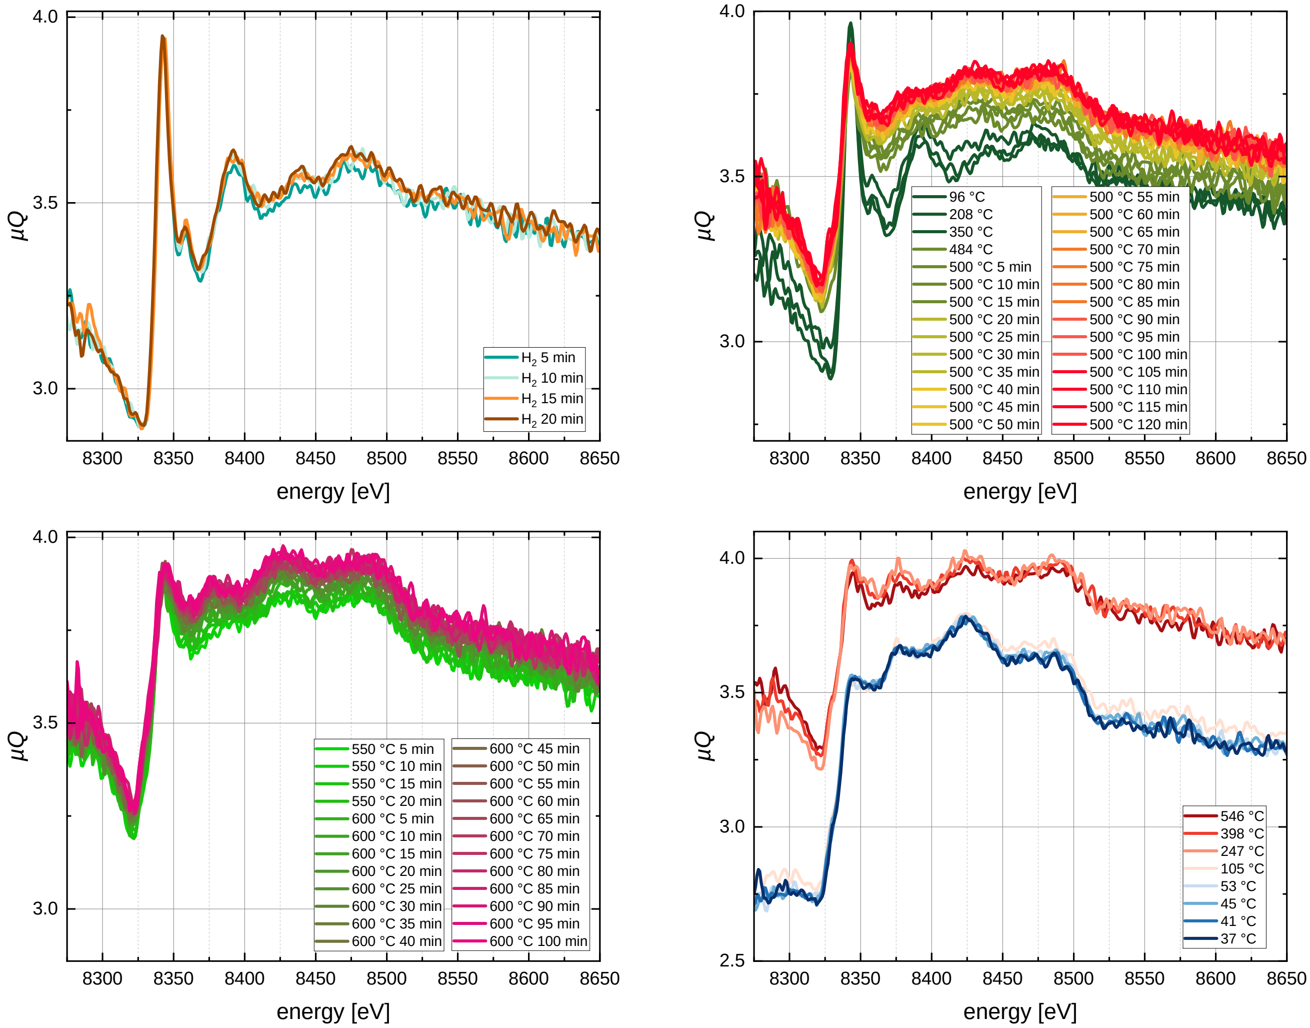


Fig. S22 Raw *in situ* XAS spectra during the reduction/activation of the catalyst 20-NiO/COK-12. Top left: during gas flow setup at RT. Top right: during heating from RT to 500 °C. Bottom left: further heating to 550 °C and 600 °C. Bottom right: during cool down to RT.

### 4.4.2 Normalized data

Fig. S23 shows the normalized spectra of the *in situ* measurement of the reduction of 20-NiO/COK-12 corresponding to the raw data shown in Fig. S22.

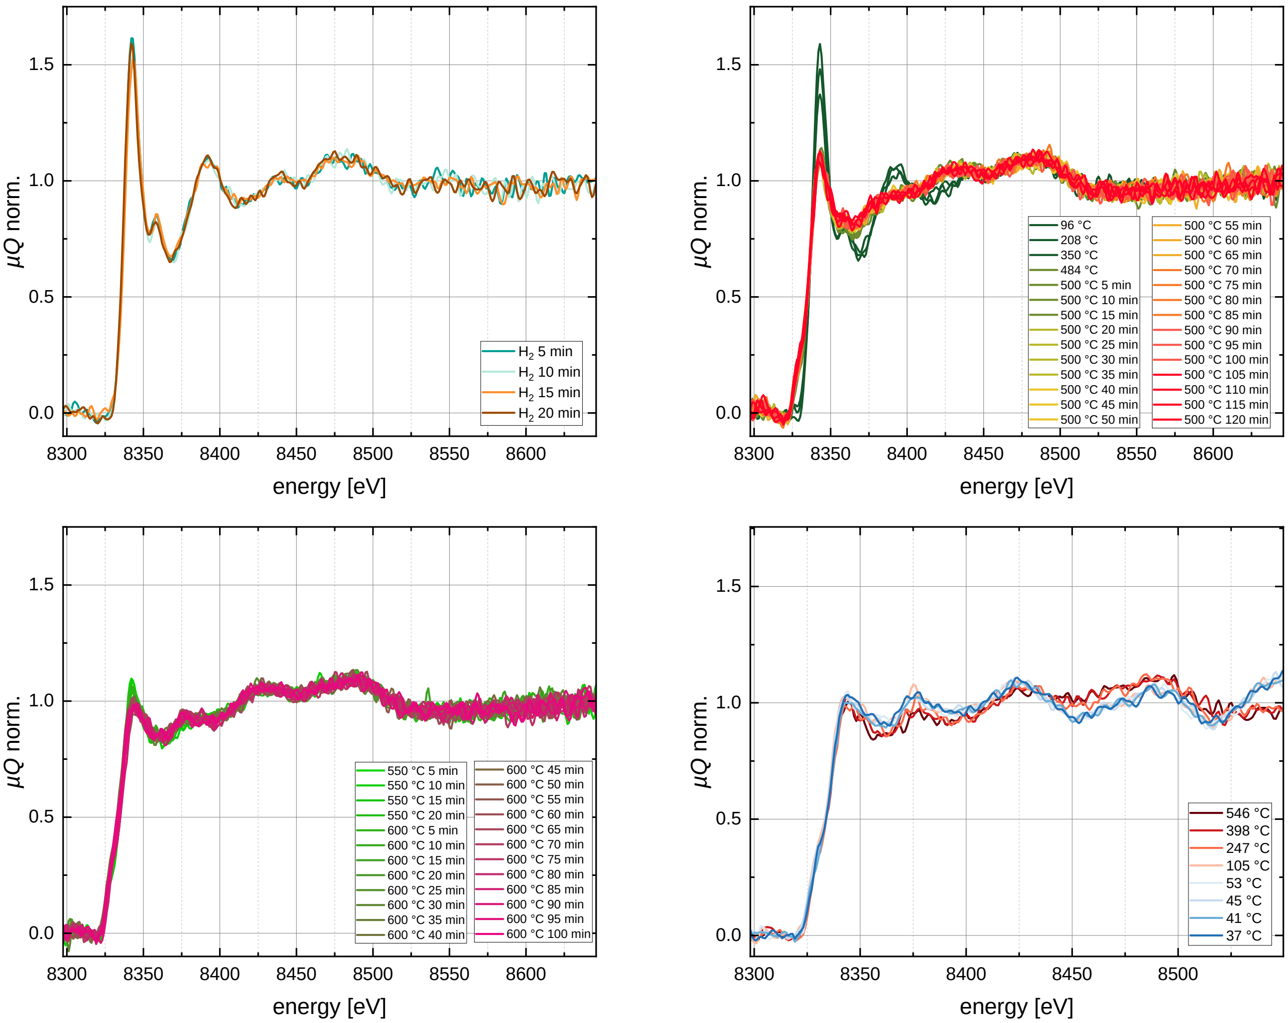


Fig. S23 Normalized *in situ* XAS spectra during the reduction/activation of the catalyst 20-NiO/COK-12. Top left: during gas flow setup at RT. Top right: during heating from RT to 500 °C. Bottom, left: further heating to 550 °C and 600 °C. Bottom, right: during cool down to RT.

### 4.4.3 Linear combination fitting

Fig. S24 shows the component fractions obtained from LCF of the *in situ* XAS measurement of 20-NiO/COK-12 during reduction. In the top panel of Fig. S24, the component fractions are plotted as a function of the applied temperature. In the bottom panel, the fractions are plotted as a function of time, with the left side corresponding to the isothermal hold at 500 °C and the right side to the subsequent increase to 600 °C.

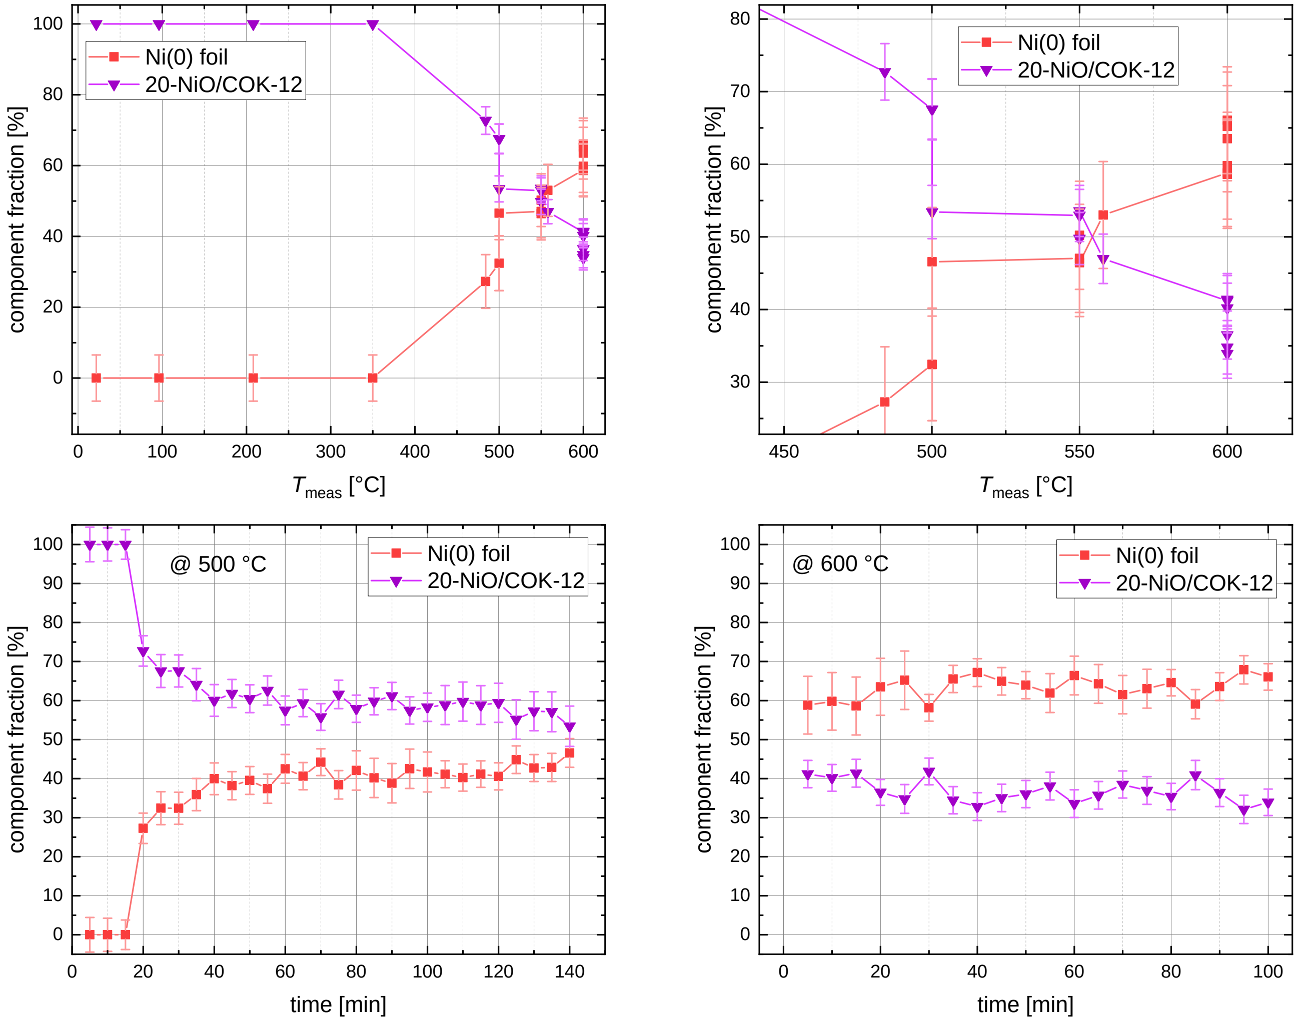


Fig. S24 Component fraction obtained by LCF of the normalized XAS spectra during *in situ* reduction/activation of 20-NiO/COK-12. Top left: From RT to 600 °C. Top right: From 450 °C to 600 °C with holding the cell at 500 °C for about 140 min and at 600 °C for about 120 min. Bottom, left: shows the evolution of the component fraction over time during heating to 500 °C and staying there for about 120 min. Bottom, right: shows the evolution of the component fraction over time during further heating to 600 °C and staying there for about 100 min.

## 5 GC measurements

This section presents the measurements obtained using the online gas chromatograph (Micro GC Fusion 2-Module System, INFICON GmbH, Cologne, Germany). Fig. S25 displays the chromatograms from Module A (left, Rt-Molsieve 5 Å) and Module B (right, Rt-Q-Bond) recorded during operation of the 20-NiO/COK-12 catalyst at 400 °C under a $H_2/CO_2$ (4:1) flow.

Fig. S26 provides a direct comparison of the catalyst measured at 350 °C under a $H_2/CO_2$ (4:1) flow before (pre) and after (post) activation/reduction. The concentrations of $CH_4$ and CO are shown alongside the temperature profile of the reactor cell. As expected, no catalytic activity is observed before activation, while clear $CH_4$ and CO formation is detected after activation.

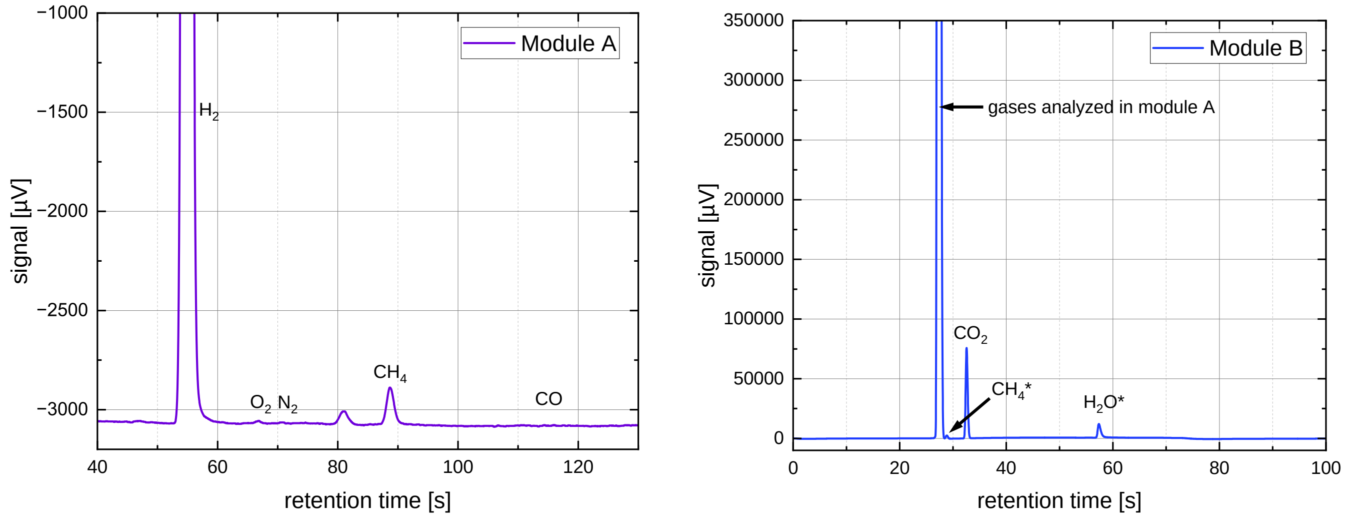


Fig. S25 Chromatograms from Module A (left, Rt-Molsieve 5 Å) and Module B (right, Rt-Q-Bond) recorded during operation of the 20-NiO/COK-12 catalyst at 400 °C under a $H_2/CO_2$ flow with a concentration ratio of 4:1. The GC was calibrated to quantify $H_2$, $N_2$, $O_2$, CO, and $CH_4$ in Module A, as well as $CO_2$ and C2–C4 hydrocarbons in Module B. * $CH_4$ and $H_2O$ signals in Module B were detectable but not calibrated and therefore not quantified.

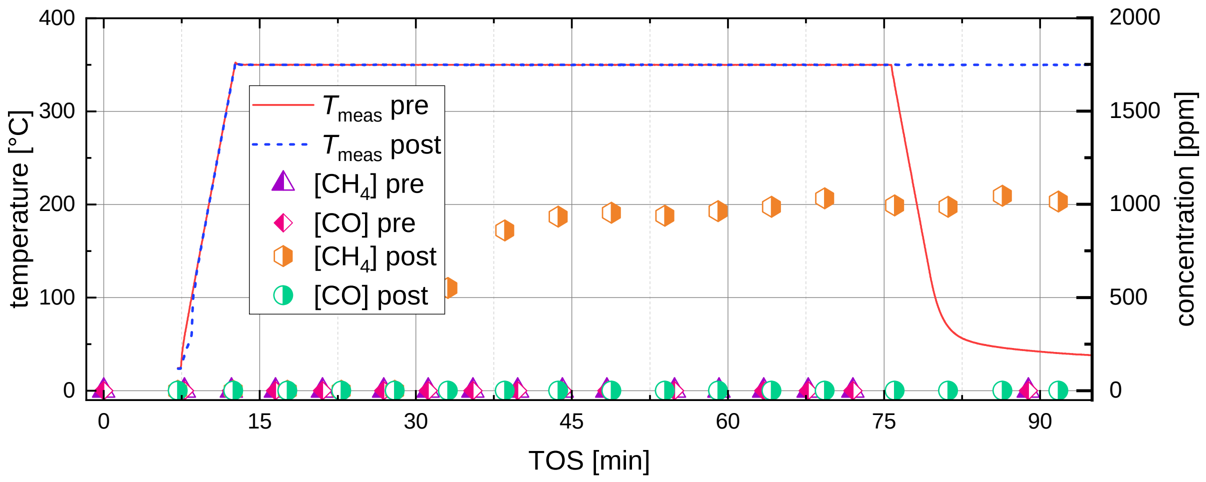


Fig. S26 Comparison of GC and temperature measurements of 20-NiO/COK-12 before (pre) and after (post) catalyst activation. The concentrations of $CH_4$ and CO are plotted over time-on-stream (TOS), alongside the corresponding temperature profile of the *in situ* cell. The data clearly demonstrate the emergence of catalytic activity – evidenced by increased $CH_4$ formation – only after activation, confirming the transformation of the catalyst into its active state.

## 6 Additional post-reduction operando experiments

Fig. S27 presents supplementary *operando* measurements of the 20-NiO/COK-12 catalyst after activation/reduction. To further evaluate the catalytic performance, the total gas flow was doubled at 350 °C (see total flow rate in panel (d)), followed by an increase in reaction temperature to 400 °C. In panel (c) of Fig. S27, the $H_2/CO_2$ ratio is shown to remain approximately 4:1 throughout the entire experiment.

As shown in Fig. S27(b), doubling the flow rate led to a decrease in the observed $CH_4$ concentration, which can be attributed to dilution of the product stream by the increased inflow of $H_2$ and $CO_2$. Conversely, increasing the reaction temperature to 400 °C resulted in a higher $CH_4$ concentration and $CO_2$ conversion, consistent with the endothermic nature of the methanation reaction and the enhanced reaction kinetics at elevated temperature.

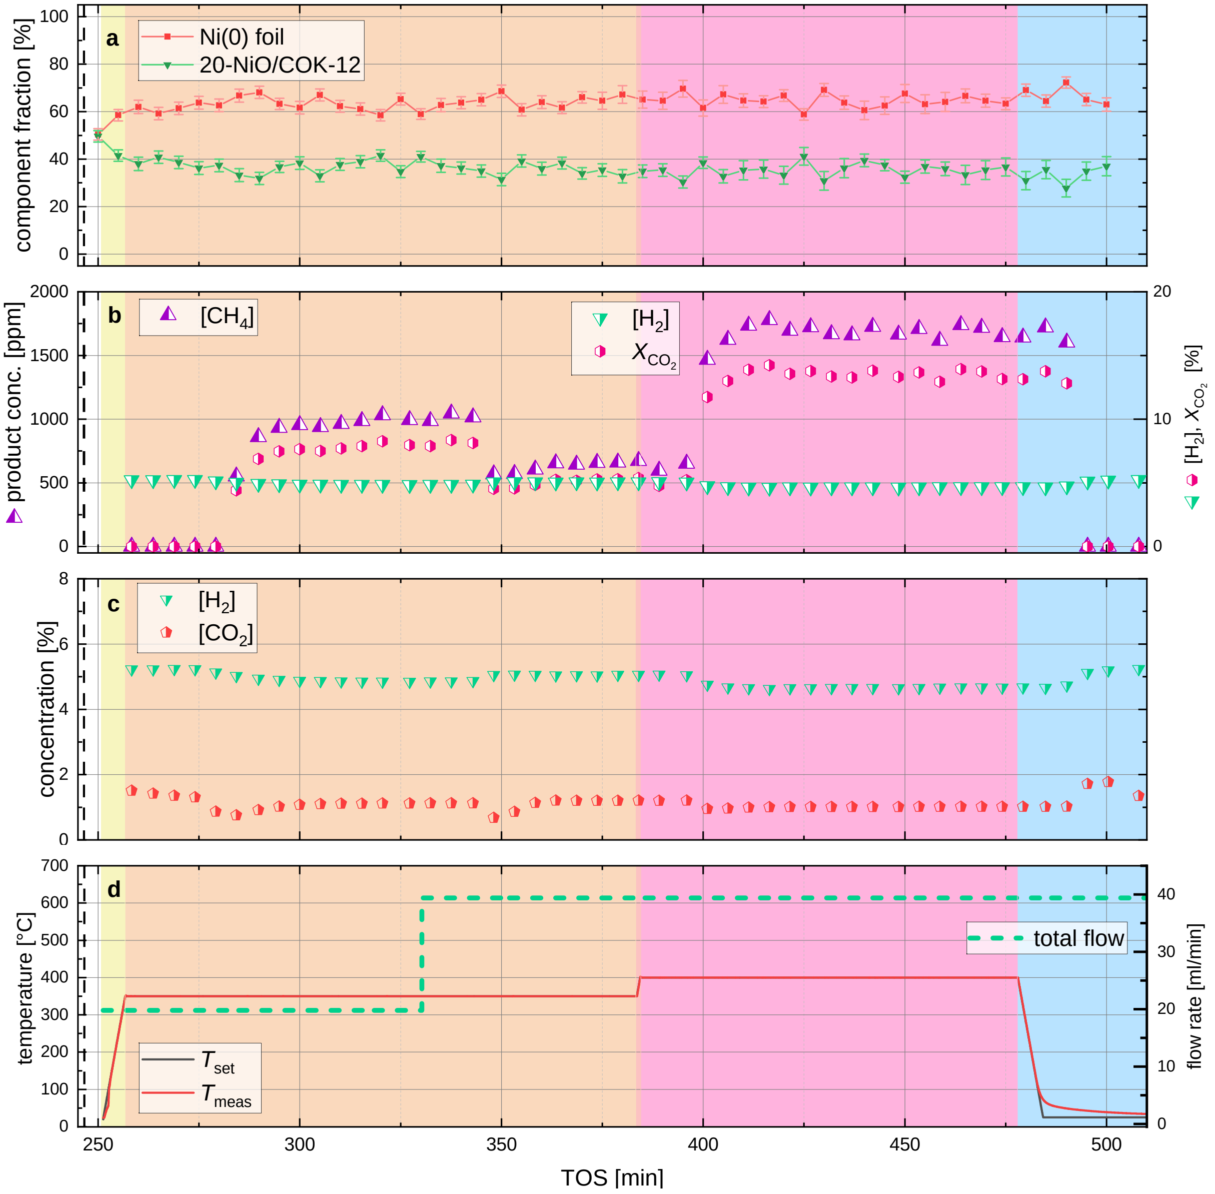


Fig. S27 Complete *operando* measurements of the 20-NiO/COK-12 catalyst after reduction. The top panel (a) displays the component fractions obtained from LCF of the XAS spectra; panel (b) shows the corresponding GC analysis of the reaction product and the $CO_2$ conversion together with the $H_2$ concentration; panel (c); and the bottom panel (d) presents the applied temperature profile and total flow rate. All data are displayed on a common cumulative time axis (time-of-stream, TOS), see pre-reduction and activation/reduction part in Fig. 6 of the main work.

# 7 X-ray source optimized for 30 keV

Fig. S28(left) shows a comparison of the empty spectra of the spectrometer aligned for Zr K-edge measurements using a molybdenum (Mo) microfocus X-ray source optimized to 15 kV and a tungsten (W) microfocus source optimized to 30 kV. The tungsten source provides a 3.7-fold increase in intensity compared to the molybdenum source, making it more suitable for measurements at higher photon energies above 15 keV.

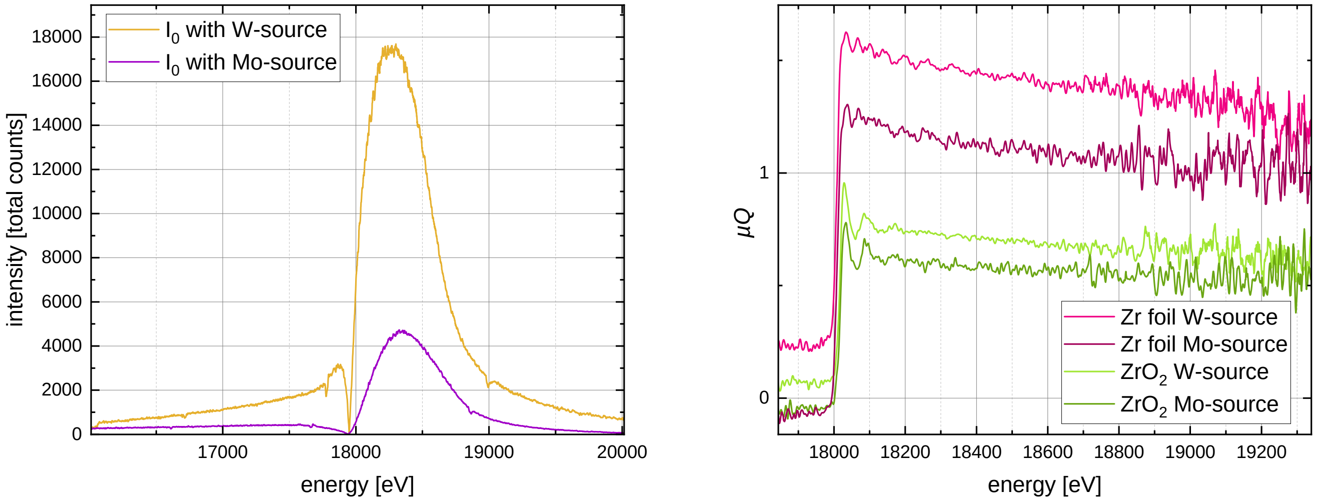


Fig. S28 Comparison of a tungsten (W) micro focus X-ray source optimized to reach 30 Watt at 30 kV – operating up to 50 kV – to the X-rays source used in this work, which is a molybdenum (Mo) micro focus source optimized to reach 30 Watt at 15 kV and operating up to 20 kV. Left: empty measurement without the sample ($I_0$) showing an 3.7 fold increase in intensity at the maximum for the W-source compared to the Mo-source. Right: Zr foil and $ZrO_2$ prepared as pellet, measured with both X-ray source showing the better SNR for the measurement performed with the W-source.

## Data availability

The raw data for this article – the raw and normalized XAS data – are available on Zenodo at `https://doi.org/10.5281/zenodo.17063731`.

## Acknowledgements

This work was partially funded by the Deutsche Forschungsgemeinschaft (DFG German Research Foundation) under Germany's Excellence Strategy – EXC2008-390540038 – UniSysCat. Part of this work was funded by the German Federal Ministry of Education and Research in the framework of the project Catlab (03EW0015A) Peter Kraus acknowledges funding from the DFG (Project No. 490703766).

## References

1 Bischoff B, Bekheet MF, Dal Molin E, Praetz S, Kanngießer B, Schomäcker R, et al. *In situ/operando* plug-flow fixed-bed cell for synchrotron PXRD and XAFS investigations at high temperature, pressure, controlled gas atmosphere and ultra-fast heating. Journal of Synchrotron Radiation. 2024 Jan;31(1):77-84. Available from: `https://doi.org/10.1107/S1600577523009591`.
